# Supplementary material for: From Occurrence to Consequence: A Comprehensive Data-driven Analysis of Building Fire Risk
Source: arXiv:2503.22689 source file (2025-03-11)
Supplement: Supplementary file 1 [file appendix_categorical_features.tex]

\begin{longtable}{>{\centering\arraybackslash}m{5cm} | >{\centering\arraybackslash}m{10cm}} 
 \caption{Fire Incident Categories and Their Sub-Categories} \label{tab:fire_category_feature} \\
    \toprule[1.5pt]
    \textbf{Variable Name} & \textbf{Sub-Category} \\
    \hline
    \endfirsthead
    \hline
    \textbf{Variable Name} & \textbf{Sub-Category} \\
    \hline
    \endhead
    \hline
    \endfoot
    Location of fire origin & 0: Means of Egress, 1: Assembly or Sales Areas (Groups of People), 2: Function Areas, 3: Technical Processing Areas, 4: Storage Areas, 5: Service Areas, 6: Service or Equipment Areas, 7: Structural Areas, 8: Transportation, Vehicle Areas (excluded), 9: Other area of origin (excluded), 10: Others, U: Unknown \\
    \hline
    First ignited item & 1: Structural Component, Finish, 2: Furniture, Utensils (includes built-in furniture), 3: Soft Goods, Wearing Apparel, 4: Adornment, Recreational Material, Signs, 5: Storage Supplies, 6: Liquids, Piping, Filters, 7: Organic Materials, 8: General Materials, 9: Other, U: Unknown \\
    \hline
    Item spread & 1: Structural Component, Finish, 2: Furniture, Utensils (includes built-in furniture), 3: Soft Goods, Wearing Apparel, 4: Adornment, Recreational Material, Signs, 5: Storage Supplies, 6: Liquids, Piping, Filters, 7: Organic Materials, 8: General Materials, 9: Other, U: Unknown \\
    \hline
    Primary action taken & 1: Fire Control or Extinguishment, 2: Search and Rescue, 3: EMS and Transport, 4: Hazardous Condition, 5: Fires, Rescues, and Hazardous Conditions, 6: Systems and Services, 7: Assistance, 8: Information, Investigation, and Enforcement, 9: Fill-in, Standby, 11: Unknown \\
    \hline
    Property usage & 1: Assembly, 2: Educational, 3: Health care, detention, and correction, 4: Residential, 5: Mercantile, business, 6: Industrial, 7: Manufacturing, Processing, 8: Storage, 9: Outside or Special Property, 10: Other, 11: None, 20: Unknown \\
    \hline
    Cause of ignition & 1: Intentional, 2: Unintentional, 3: Failure of equipment of heat source, 4: Act of nature, 5: Cause under investigation, U: Cause underdetermined after investigation \\
    \hline
    Human factors contributing to ignition & 1: Asleep, 2: Possibly impaired by alcohol or drugs, 3: Unattended person, 4: Possibly mentally disabled, 5: Physically disabled, 6: Multiple persons involved \\
    \hline
    Heat source & 1: Operating equipment, 2: Hot or smolder object, 3: Explosives, 4: Other open flame or smoking materials, 5: Chemical natural heat source, 6: Heat spread from another fire (excluded), 7: Multiple sources, 8: Other, U: Unknown \\
    \hline
    Detector & 1: Detector presents, 2: No detector, 3: Unknown \\
    \hline
    AES & 1: AES present, 2: AES partially present, N: No AES, U: Unknown\\

\bottomrule[1.5pt]

\end{longtable}
